# Supplementary material for: AutoInt: Automatic Feature Interaction Learning via Self-Attentive Neural Networks
Source: arXiv:1810.11921 source file (2019-08-23)
Supplement: Supplementary file 1 [file appendix.tex]

\clearpage

\appendix
\appendixpage

\section{Data}
We use four public real-world data sets in this paper, and the link for each data set is available in Section~\ref{subsubsec::data}.
For all datasets, we randomly select 80\% of all samples for training and randomly split the rest into validation and test sets of equal size. Since Criteo, Avazu and KDD12 data sets are too large to fit into the memory, we randomly split each of them into eight files and load small files into memory one by one during training.

\section{Implementation Details}
As a supplement to Section~\ref{sec::impl}, we next explain how we deal with multi-valued input during implementation and present parameter settings that produce experimental results in this paper.

%\subsection{Parameter Setting}
%To encourage the reproducibility of the experiments, 
\subsection{Multi-Value Field}
In Section~\ref{sec::input_layer}, we assume each input feature field is single-valued and $\mathbf{x_i}$ is either an one-hot vector or a scalar. However, there are also some cases where the input feature is multi-valued. For example, MovieLens-1M data has a feature field \emph{Genre}, which describes the types of a movie and may be multi-valued. To be compatible with multi-valued inputs, we slightly modify the Equation~\ref{eq::categorical_feature} and map the multi-valued input into a multi-hot vector $\mathbf{x_i}$. Afterward, the multi-valued field is represented as the average of corresponding feature embedding vectors:
%In some datasets, there could be multi-value fields (e.g. A movie belongs to multiple genres -- Action, Adventure and Thriller). We map the categorical feature into a multi-hot vector, and use the average of corresponding feature embedding vectors to represent this field:
\begin{equation}
\mathbf{e_i} = \frac{1}{q}\mathbf{V_i}\mathbf{x_i},
\end{equation}
where $q$ is the number of values that a sample has for $i$-th field and $\mathbf{x_i}$ is a multi-hot vector.

%belongs, or the Lasso regularization of $\mathbf{x_i}$. It can be written as:
%\begin{equation}
%\mathbf{e_i} = %\frac{\mathbf{V_i}\mathbf{x_i}}%{\left\|\mathbf{x_i}\right\|_1},
%\end{equation}

\subsection{Parameter Setting}
We now introduce the parameter settings used in our experiment. First, we list all the constant parameters which are fixed during experiments in Table~\ref{tab::const_param}.
%\textcolor{red}{please check the notation, especially for L,D,K}

\begin{table}[htbp]
    \centering
    
    \begin{threeparttable}
    \caption{Constant parameter setting.}\label{tab::const_param}
    \begin{tabular}{c|c|c}
    \toprule
        PARAM & Description & Value \\
        \midrule
        $Lr$ & Initial learning rate for Adam~\cite{kingma2014adam}. & 0.001 \\
        $BS$ & Batch size for training. & 1024 \\
        $d$ & Dimension of feature embedding . & 16 \\
        $d'$ & Number of hidden units of each head. & 32 \\
        $H$ & Number of total heads. & 2 \\
        $L$ & Number of interacting layers. & 3 \\
        $D^{\clubsuit}$ & Number of feed-forward layers. & 2 \\
        $K^{\clubsuit}$ & Number of hidden units for each layer. & 400 \\
    \bottomrule
    \end{tabular}
    %\begin{}
    \begin{tablenotes}
    \centering
      \small
      \item $\clubsuit$: only applicable for joint training models in Section~\ref{sec::joint}.
    \end{tablenotes}
    \end{threeparttable}
\end{table}

The only tuned hyper-parameter is dropout rate. We use dropout~\cite{srivastava2014dropout} to prevent overfitting on small data set, i.e., MovieLens-1M data.
Following~\cite{he2017neural,xiao2017attentional,guo2017deepfm}, we use different dropout rate for different layer which is determined by grid search. The search space is $\{0, 0.1, \cdots, 0.9\}$. The optimal dropout rate is 0.4 for interacting layer and 0.1 for other layers (embedding layer and feed-forward layer in joint training).

%\section{More results}
%We can present performance w.r.t. different number of attention head in this section. If you think it's too time-consuming, results on two datasets are acceptable. 

\section{Environment}
We conduct experiments in the environment with following configurations: %\textcolor{red}{config for 244, please check}
\begin{itemize}
    \item CPU: Intel(R) Xeon(R) CPU E5-2650 v4 @ 2.20GHz.
    \item Memory: 128GB.
    \item GPU: NVIDIA TITAN Xp, 12GB.
    \item Software: Ubuntu v16.04.3, Tensorflow v1.4.1.
\end{itemize}
